# Supplementary material for: Core Electron Binding Energies in Solids from Periodic All-Electron $\Delta$-Self-Consistent-Field Calculations
Source: arXiv:2104.06356 ancillary file (2021-08-24)
Supplement: Supplementary file 1 [file Supplementary_information_v1.pdf]

# Experimental core electron binding energies

For metals and graphite, the binding energies are given relative to the Fermi level. For insulators, values referenced to the valence band maximum are reported.

## Li 1s in lithium metal

| | |
|---|---|
| Shek, M. *et al.*, Surf. Sci. **234**, 324 (1990) | 55.1 eV |
| Contour, J. *et al.*, J. Microsc. Spect. Elec. **4**, 483 (1979) | 54.6 eV |
| Wertheim, G. *et al.*, Solid State Commun. **33**, 1127 (1980) | 54.9 eV |
| Kowalczyk, S.P. *et al.*, Phys. Rev. B **8**, 3583 (1973) | 54.8 eV |
| Average: | **54.85 eV** |

## Be 1s in beryllium metal

| | |
|---|---|
| Powell, C.J., Appl. Surf. Sci. **89**, 141 (1995) * | 111.85 eV |
| * recommended reference value based on three different measurements | |
| Average: | **111.85 eV** |

## Na 1s in sodium metal

| | |
|---|---|
| Kowalczyk, S.P. *et al.*, Phys. Rev. B **8**, 3583 (1973) | 1071.7 eV |
| Barrie, A. *et al.*, J. Electron. Spectrosc. **7**, 1 (1975) | 1071.8 eV |
| Citrin, P.H., Phys. Rev. B **8**, 5545 (1973) | 1071.76 eV |
| Average: | **1071.75 eV** |

## Na 2p in sodium metal

| | |
|---|---|
| Kowalczyk, S.P. *et al.*, Phys. Rev. B **8**, 3583 (1973) | 30.4 eV |
| Barrie, A. *et al.*, J. Electron. Spectrosc. **7**, 1 (1975) | 30.6 eV |
| Citrin, P.H., Phys. Rev. B **8**, 5545 (1973) | 30.52 eV |
| Average: | **30.51 eV** |

### Mg 1s in magnesium metal

| | |
|---|---|
| Jennison, D.R. *et al.*, Solid State Phys. **17**, 3701 (1984) | 1303.2 eV |
| Yoshimura, K. *et al.*, Jpn. J. Appl. Phys. **46**, 4260 (2007) | 1303.5 eV |
| Ley, L. *et al.*, Phys. Rev. B **11**, 600 (1975) | 1303.0 eV |
| Peng, X. *et al.*, Surf. Sci. **195**, 103 (1988) | 1303.3 eV |
| Darrah Thomas, T. *et al.*, Phys. Rev. B **33**, 5406 (1986) | 1303.2 eV |
| Average: | **1303.24 eV** |

### Mg 2p in magnesium metal

| | |
|---|---|
| Powell, C.J., Appl. Surf. Sci. **89**, 141 (1995) * | 49.79 eV |
| * recommended reference value based on three different measurements | |
| Average: | **49.79 eV** |

### C 1s in graphite

| | |
|---|---|
| Kieser, J. *et al.*, Appl. Phys. **9**, 315 (1976) | 284.31 eV |
| Johansson, G. *et al.*, J. Electron. Spectrosc. **2**, 295 (1973) | 284.3 eV |
| Xie, Y. *et al.*, Surf. Sci. Spectra **1**, 367 (1992) | 284.64 eV |
| Harmin, K., *et al.*, Phys. Scr. **1**, 277 (1970) | 284.3 eV |
| Estrade-Szwarckopf, H., *et al.*, J. Phys. Chem. Solids **53**, 419 (1992) | 284.5 eV |
| Average: | **284.41 eV** |

### Be 1s in BeO

| | |
|---|---|
| Hamrin, K. *et al.*, Phys. Scr. **1**, 277 (1970) | 109.8 eV |
| Koh, D. *et al.*, J. Vac. Sci. Technol. B **37**, 041206 (2019) | 110.2 eV |
| Average: | **110.00 eV** |

### O 1s in BeO

| | |
|---|---|
| Hamrin, K. *et al.*, Phys. Scr. **1**, 277 (1970) | 527.7 eV |
| Average: | **527.70 eV** |

**B 1s in hex-BN**

| | |
|---|---|
| Hamrin, K. *et al.*, Phys. Scr. **1**, 277 (1970) | 188.4 eV |
| Henck, H. *et al.*, Phys. Rev. B **95**, 085410 (2017) | 188.3 eV |
| Average: | **188.35 eV** |

**N 1s in hex-BN**

| | |
|---|---|
| Hamrin, K. *et al.*, Phys. Scr. **1**, 277 (1970) | 396.1 eV |
| Henck, H. *et al.*, Phys. Rev. B **95**, 085410 (2017) | 395.9 eV |
| Average: | **396.00 eV** |

**C 1s in diamond**

| | |
|---|---|
| Gaowei, M. *et al.*, Appl. Phys. Lett. **100**, 201606 (2012) | 284.44 eV |
| McFeely, F.R. *et al.*, Phys. Rev. B **9**, 5268 (1974) | 283.8 eV |
| Kono, S. *et al.*, Jpn. J. Appl. Phys. **53**, 05FP03 (2014) | 284.01 eV |
| Maier, F. *et al.*, Phys. Rev. B **64**, 165411 (2001) | 283.9 eV |
| Average: | **284.04 eV** |

**Si 2p in β-SiC**

| | |
|---|---|
| Bermudez, V.M., J. Appl. Phys. 63, 4951 (1988) | 99.1 eV |
| King, S.W. et al., J. Electron. Mater. 28, L34 (1999) | 99.3 eV |
| Average: | **99.20 eV** |

**C 1s in β-SiC**

| | |
|---|---|
| Bermudez, V.M., J. Appl. Phys. 63, 4951 (1988) | 281.9 eV |
| Waldrop, J.R. et al., Appl. Phys. Lett. 56, 557 (1990) | 281.45 eV |
| King, S.W. et al., J. Electron. Mater. 28, L34 (1999) | 281.3 eV |
| Average: | **281.55 eV** |

**Si 2p in silicon**

| | |
|---|---|
| Yu, E.T. et al., Appl. Phys. Lett. 56, 569 (1990) | 98.95 eV |
| Puthenkovilakam, R. et al., Appl. Phys. Lett. 84, 1353 (2004) | 99.1 eV |
| Average: | **99.03 eV** |

# High frequency (optical) dielectric constants

| Material | Reference | $\varepsilon_r$ |
|---|---|---|
| BeO | Gaskins, J.T. *et al.*, ECS J. Solid State Sci. Technol. **6** N189 (2017) | 2.9 |
| hex-BN | Geick. R, *et al.*, Phys. Rev. **146**, 543 (1966) *<br>* averaged over in-plane and out-of-plane directions. | 4.67 |
| Diamond | Madelung, O. et al., “Semiconductors: Group IV Elements, IV-IV and III-V Compounds. Part a – Lattice Properties”, Springer-Verlag Berlin Heidelberg (2001) | 5.7 |
| β-SiC | Patrick, L. et al., Phys. Rev. B 2, 2255 (1970) | 6.52 |
| Silicon | Madelung, O. et al., “Semiconductors: Group IV Elements, IV-IV and III-V Compounds. Part a – Lattice Properties”, Springer-Verlag Berlin Heidelberg (2001) | 11.7 |

# Extrapolation of calculated core electron binding energies

### Li 1s in lithium metal

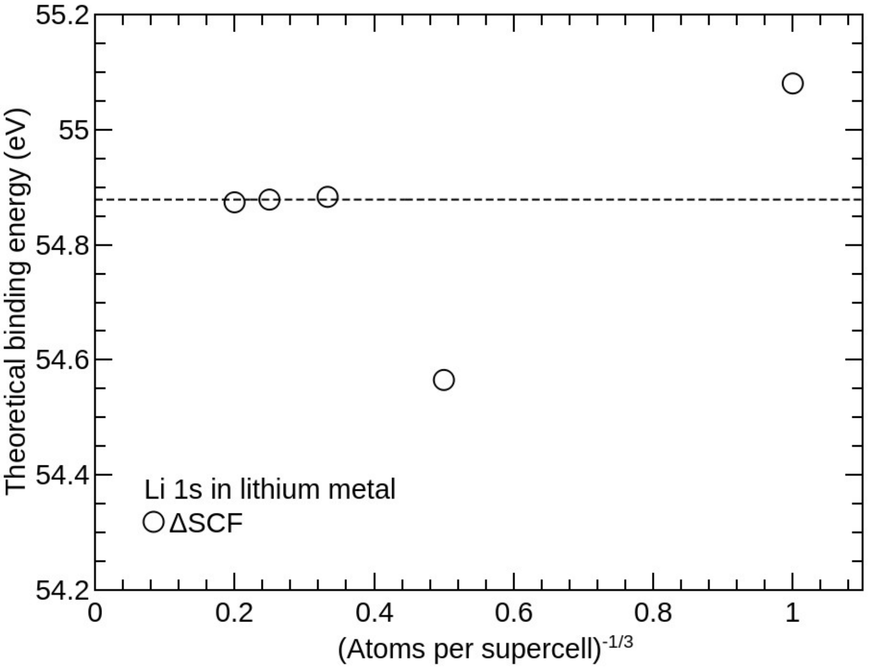

**Be 1s in beryllium metal**

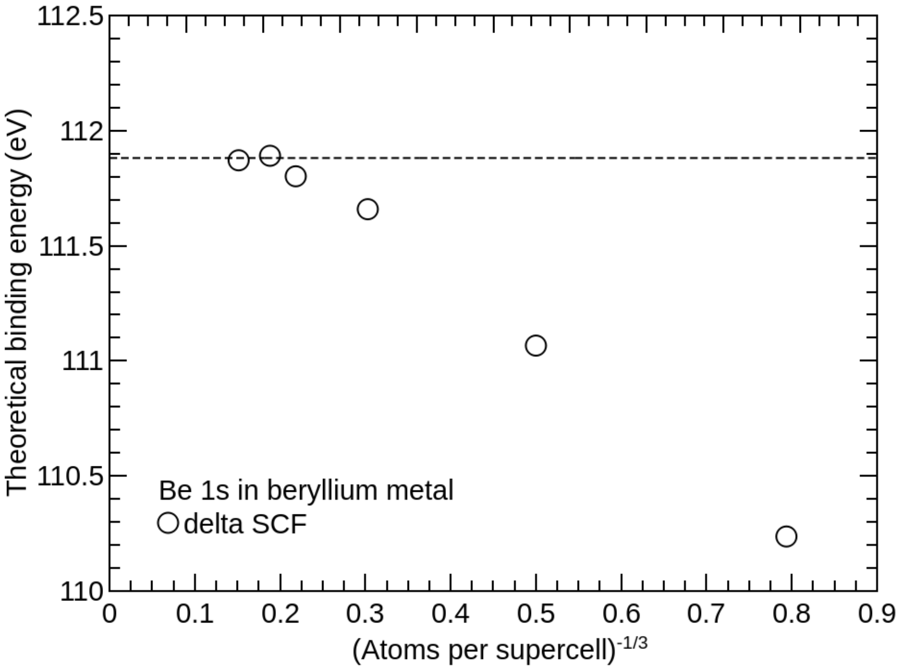


**Na 1s in sodium metal**

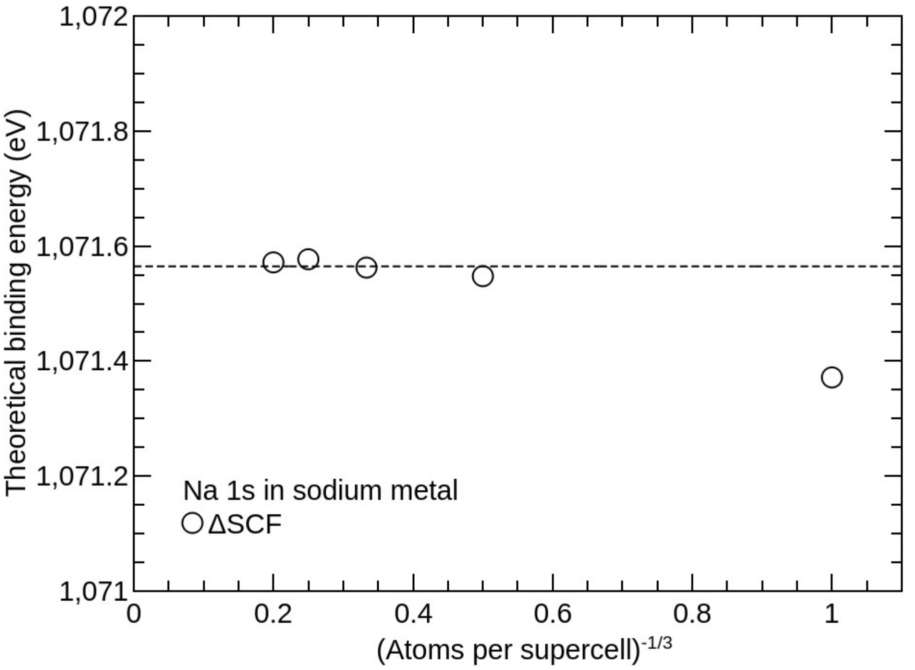

## Na 2p in sodium metal

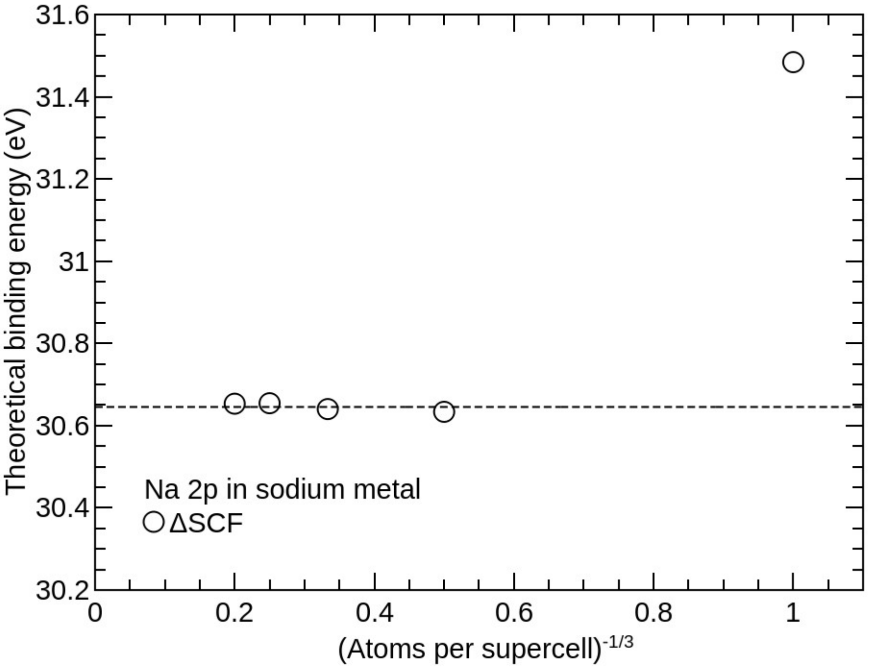


## Mg 1s in magnesium metal

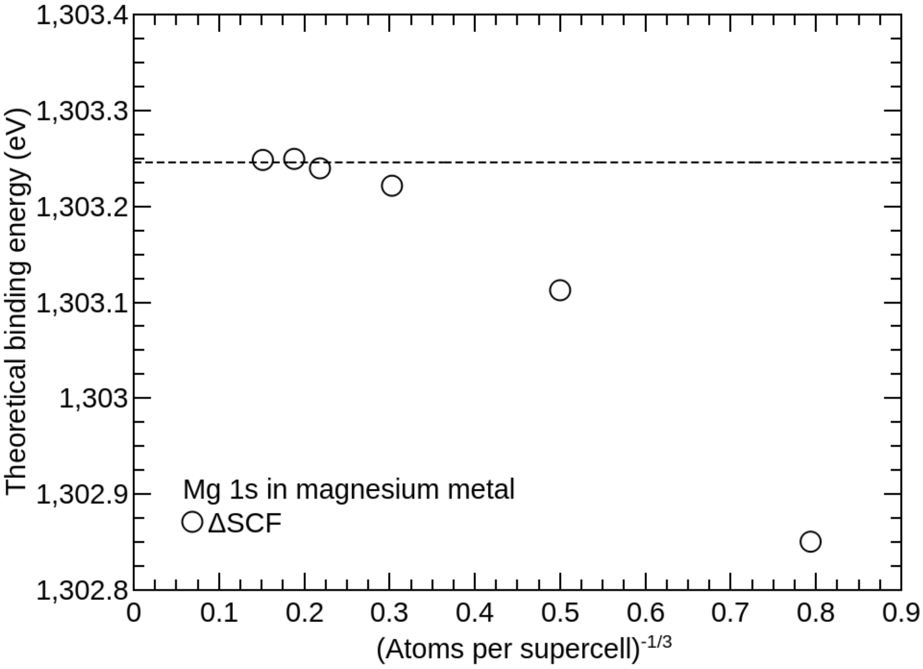

## Mg 2p in magnesium metal

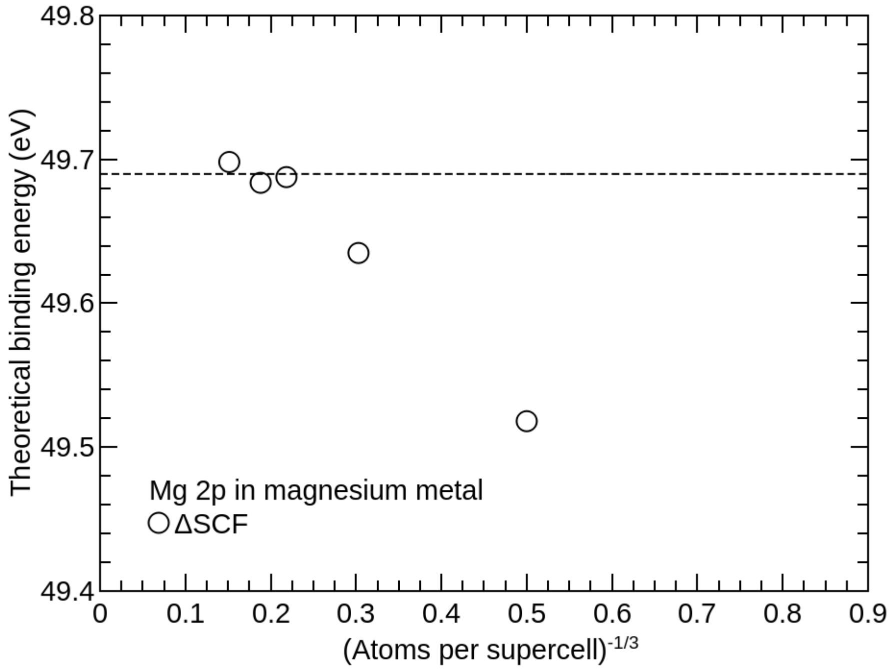


## C 1s in graphite

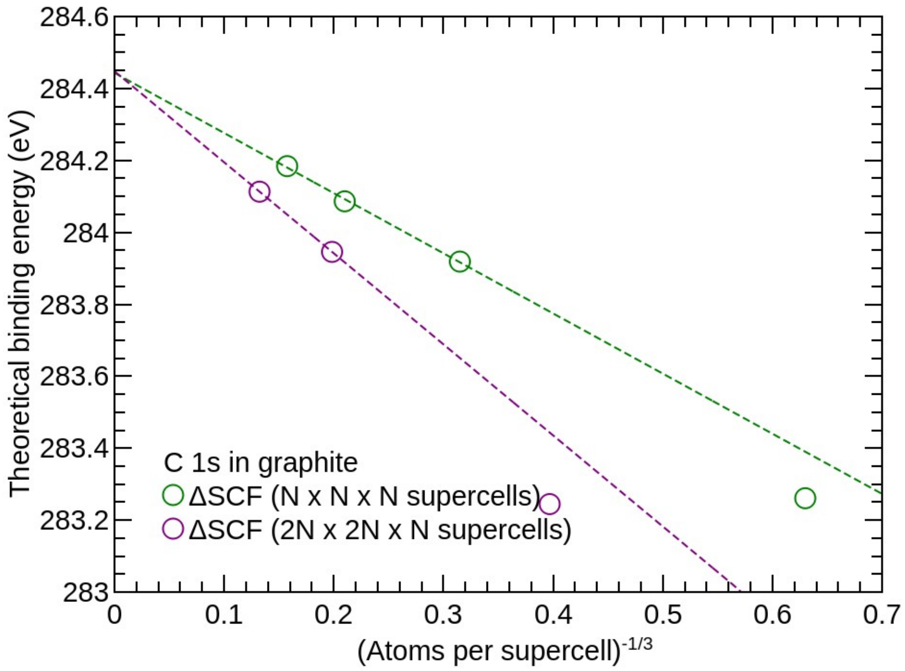

**Be 1s in BeO**

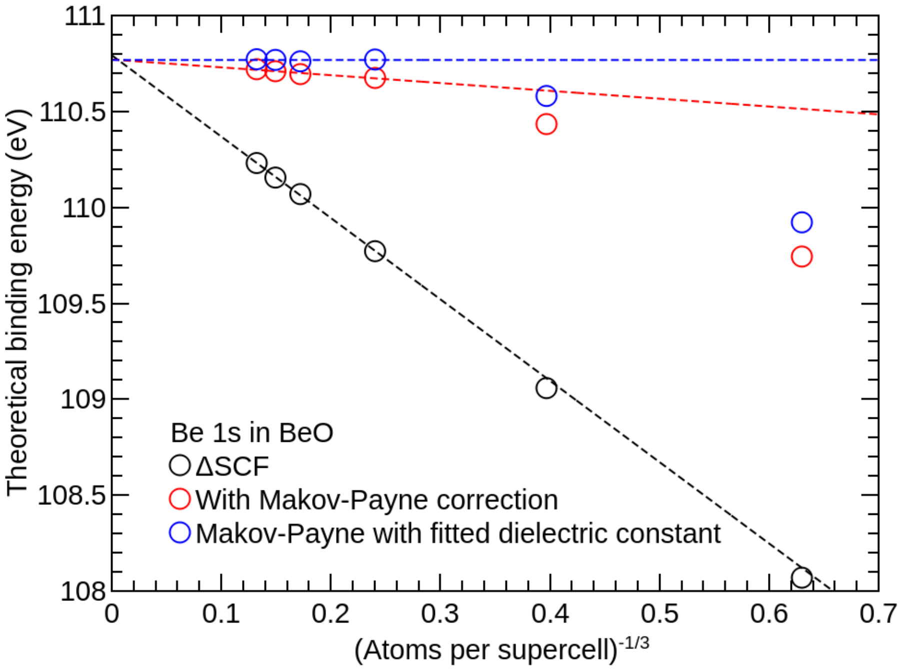


**O 1s in BeO**

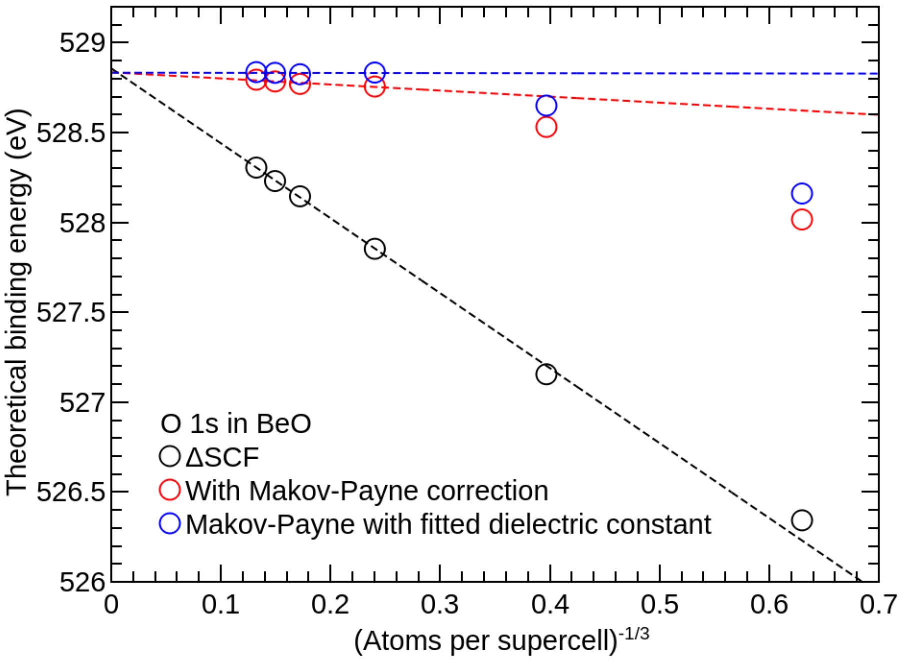

**B 1s in hex-BN**

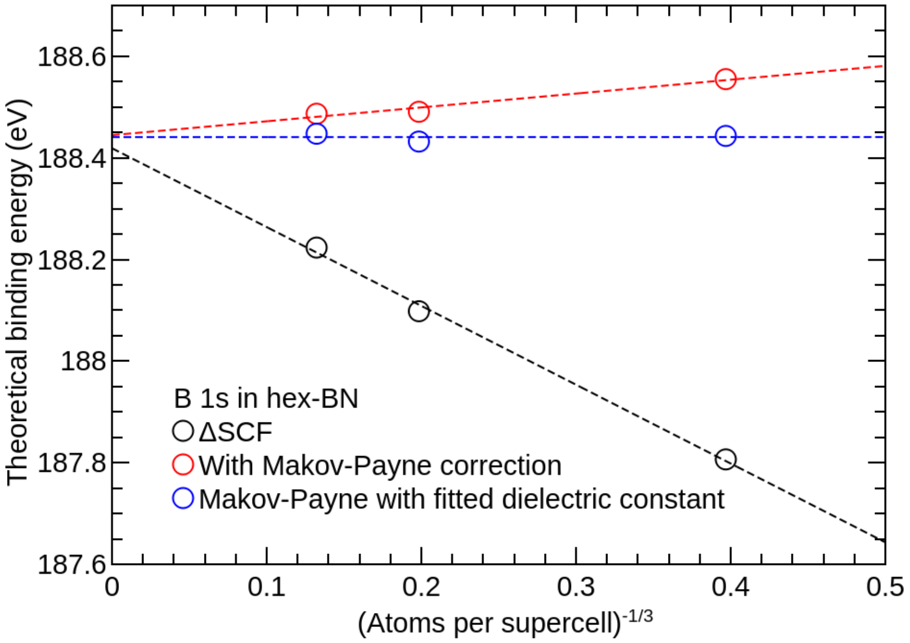


**N 1s in hex-BN**

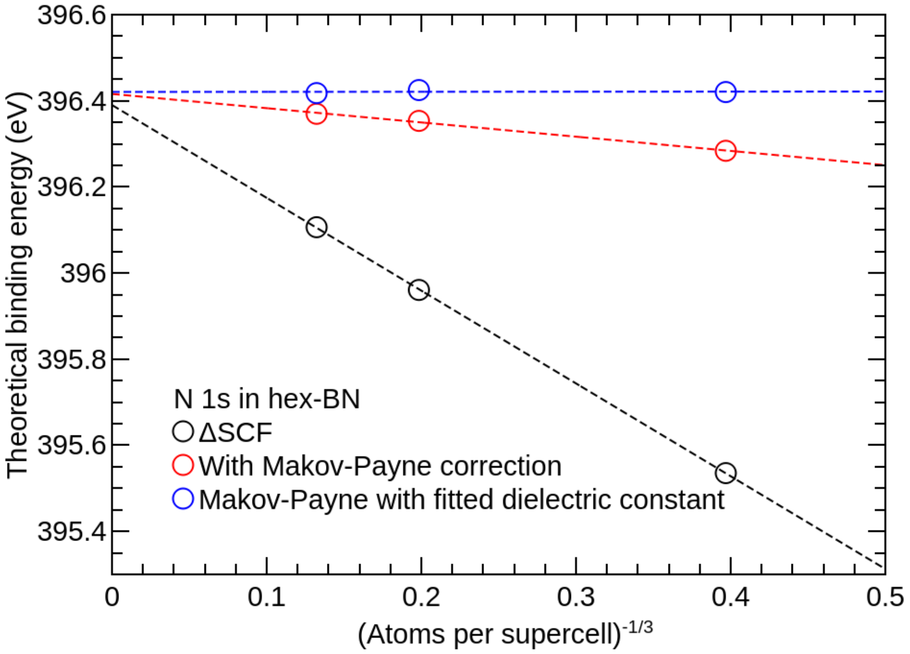

**C 1s in diamond**

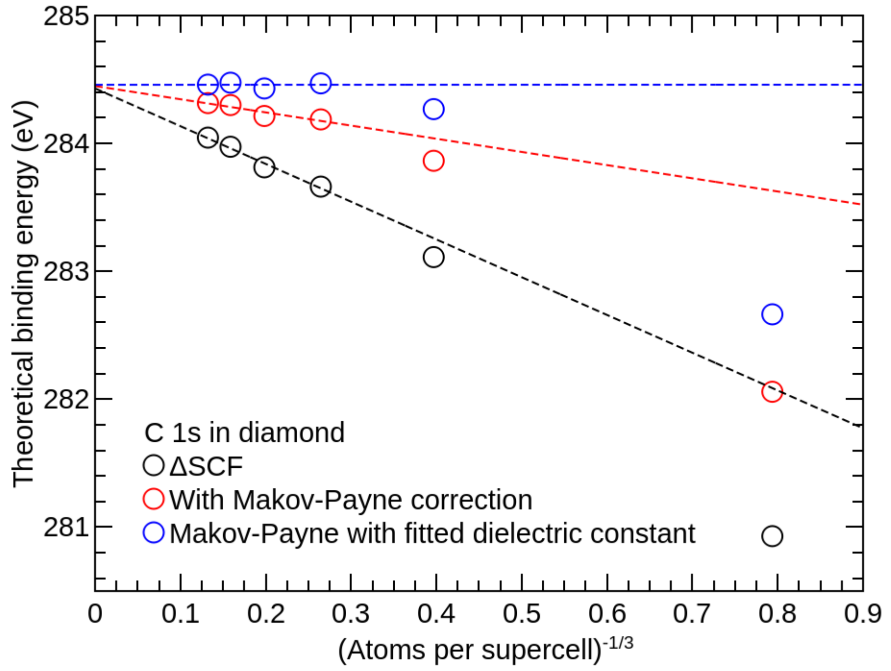


**Si 2p in β-SiC**

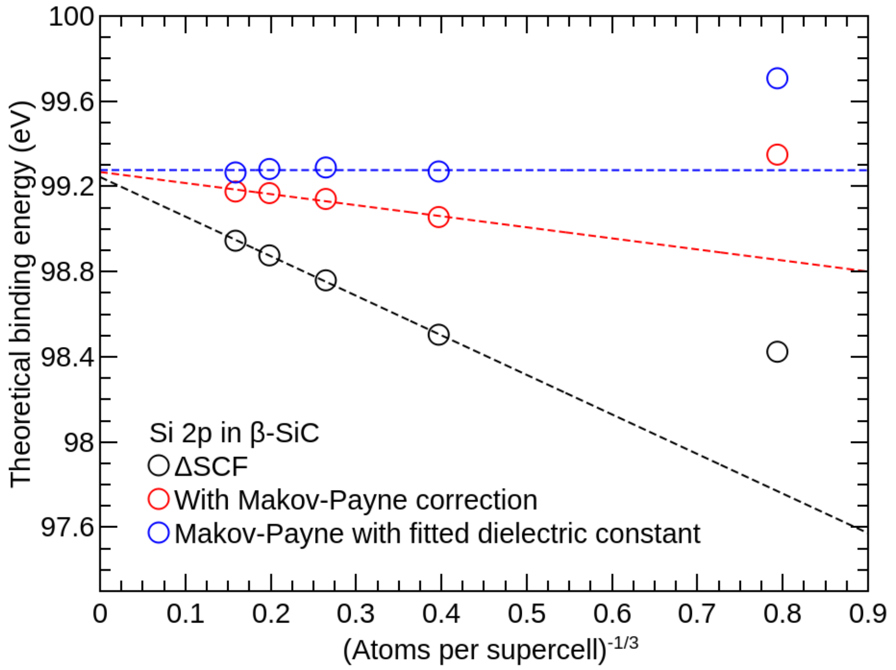

**C 1s in β-SiC**

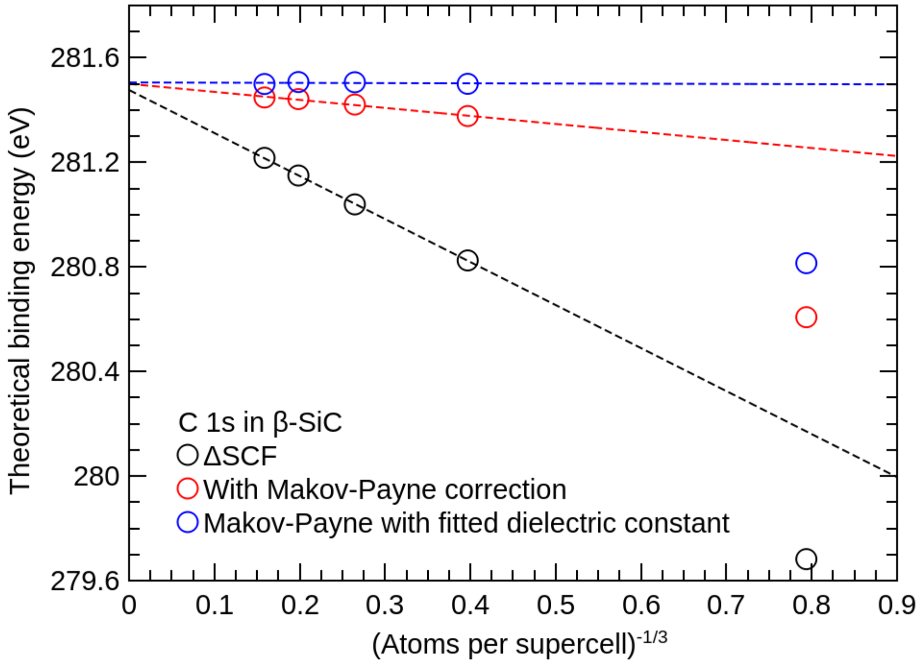


**Si 2p in silicon**

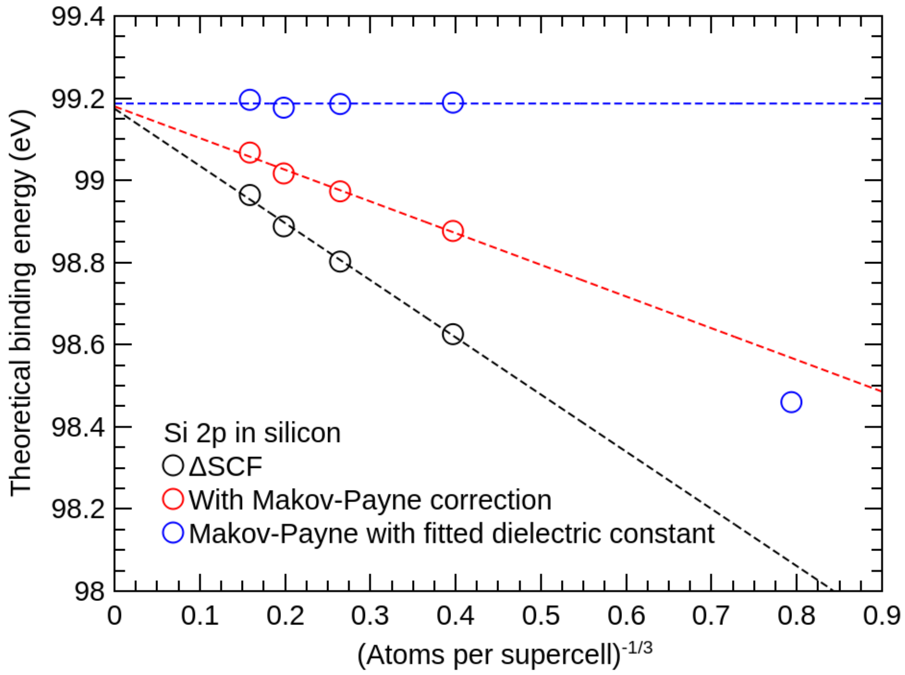

# k-point grids, finite size corrections, and numerical results

Finite size corrections are only given (and applied) for insulators. “MP corr. BE” stands for the calculated binding energy with the Makov-Payne correction using the experimental (optical) dielectric constant. “MP (fit ε) corr. BE” stands for the calculated binding energy with the Makov-Payne correction using a fitted dielectric constant that makes the binding energy independent of supercell size for the largest supercells.

### Li 1s in lithium metal

| Supercell | Atoms | k-grid | ΔSCF (eV) |
|---|---|---|---|
| 1×1×1 | 1 | 30×30×30 | 55.08 |
| 2×2×2 | 8 | 15×15×15 | 54.57 |
| 3×3×3 | 27 | 10×10×10 | 54.88 |
| 4×4×4 | 64 | 8×8×8 | 54.88 |
| 5×5×5 | 125 | 6×6×6 | 54.87 |
| Extrapolated value: | | | 54.88 |

### Be 1s in beryllium metal

| Supercell | Atoms | k-grid | ΔSCF (eV) |
|---|---|---|---|
| 1×1×1 | 2 | 48×48×32 | 110.24 |
| 2×2×1 | 8 | 24×24×32 | 111.07 |
| 3×3×2 | 36 | 16×16×16 | 111.66 |
| 4×4×3 | 96 | 12×12×11 | 111.80 |
| 5×5×3 | 150 | 10×10×11 | 111.89 |
| 6×6×4 | 288 | 8×8×8 | 111.87 |
| Extrapolated value: | | | 111.88 |

### Na 1s in sodium metal

| Supercell | Atoms | k-grid | ΔSCF (eV) |
|---|---|---|---|
| 1×1×1 | 1 | 30×30×30 | 1071.37 |
| 2×2×2 | 8 | 15×15×15 | 1071.55 |
| 3×3×3 | 27 | 10×10×10 | 1071.56 |
| 4×4×4 | 64 | 8×8×8 | 1071.58 |
| 5×5×5 | 125 | 6×6×6 | 1071.57 |
| Extrapolated value: | | | 1071.56 |

**Na 2p in sodium metal**

| Supercell | Atoms | k-grid | ΔSCF (eV) |
|---|---|---|---|
| 1×1×1 | 1 | 30×30×30 | 31.48 |
| 2×2×2 | 8 | 15×15×15 | 30.63 |
| 3×3×3 | 27 | 10×10×10 | 30.64 |
| 4×4×4 | 64 | 8×8×8 | 30.65 |
| 5×5×5 | 125 | 6×6×6 | 30.65 |
| Extrapolated value: | | | 30.65 |

**Mg 1s in magnesium metal**

| Supercell | Atoms | k-grid | ΔSCF (eV) |
|---|---|---|---|
| 1×1×1 | 2 | 48×48×32 | 1302.85 |
| 2×2×1 | 8 | 24×24×32 | 1303.11 |
| 3×3×2 | 36 | 16×16×16 | 1303.22 |
| 4×4×3 | 96 | 12×12×11 | 1303.24 |
| 5×5×3 | 150 | 10×10×11 | 1303.25 |
| 6×6×4 | 288 | 8×8×8 | 1303.25 |
| Extrapolated value: | | | 1303.25 |

**Mg 2p in magnesium metal**

| Supercell | Atoms | k-grid | ΔSCF (eV) |
|---|---|---|---|
| 1×1×1 | 2 | 48×48×32 | 50.16 |
| 2×2×1 | 8 | 24×24×32 | 49.52 |
| 3×3×2 | 36 | 16×16×16 | 49.63 |
| 4×4×3 | 96 | 12×12×11 | 49.69 |
| 5×5×3 | 150 | 10×10×11 | 49.68 |
| 6×6×4 | 288 | 8×8×8 | 49.70 |
| Extrapolated value: | | | 49.69 |

**C 1s in graphite**

| Supercell | Atoms | k-grid | ΔSCF (eV) |
|---|---|---|---|
| 1×1×1 | 4 | 36×36×12 | 283.26 |
| 2×2×2 | 32 | 18×18×6 | 283.92 |
| 3×3×3 | 108 | 12×12×4 | 284.09 |
| 4×4×4 | 256 | 9×9×3 | 284.18 |
| 2×2×1 | 16 | 18×18×12 | 283.24 |
| 4×4×2 | 128 | 9×9×6 | 283.95 |
| 6×6×3 | 432 | 6×6×4 | 284.11 |
| Extrapolated value: | | | 284.44 |

**Be 1s in BeO**

| Supercell | Atoms | k-grid | $q^2\alpha/2L$ (eV) | ΔSCF (eV) | MP corr. BE (eV) | MP (fit ε) corr. BE (eV) |
|---|---|---|---|---|---|---|
| 1×1×1 | 4 | 30×30×18 | 4.85 | 108.07 | 109.74 | 109.92 |
| 2×2×1 | 16 | 15×15×18 | 3.99 | 109.06 | 110.43 | 110.58 |
| 3×3×2 | 72 | 10×10×9 | 2.62 | 109.77 | 110.67 | 110.77 |
| 4×4×3 | 196 | 8×8×6 | 1.81 | 110.07 | 110.69 | 110.76 |
| 5×5×3 | 300 | 6×6×6 | 1.61 | 110.16 | 110.71 | 110.77 |
| 6×6×3 | 432 | 5×5×6 | 1.42 | 110.23 | 110.72 | 110.77 |
| Extrapolated values: | | | | 110.79 | 110.77 | 110.77 |
| Experimental dielectric constant = 2.9, fitted dielectric constant = 2.62 | | | | | | |

**O 1s in BeO**

| Supercell | Atoms | k-grid | $q^2\alpha/2L$ (eV) | ΔSCF (eV) | MP corr. BE (eV) | MP (fit ε) corr. BE (eV) |
|---|---|---|---|---|---|---|
| 1×1×1 | 4 | 30×30×18 | 4.85 | 526.34 | 528.02 | 528.16 |
| 2×2×1 | 16 | 15×15×18 | 3.99 | 527.16 | 528.53 | 528.65 |
| 3×3×2 | 72 | 10×10×9 | 2.62 | 527.85 | 528.76 | 528.83 |
| 4×4×3 | 196 | 8×8×6 | 1.81 | 528.15 | 528.77 | 528.82 |
| 5×5×3 | 300 | 6×6×6 | 1.61 | 528.23 | 528.78 | 528.83 |
| 6×6×3 | 432 | 5×5×6 | 1.42 | 528.31 | 528.79 | 528.84 |
| Extrapolated values: | | | | 528.86 | 528.83 | 528.83 |
| Experimental dielectric constant = 2.9, fitted dielectric constant = 2.67 | | | | | | |

**B 1s in hex-BN**

| Supercell | Atoms | k-grid | $q^2\alpha/2L$ (eV) | ΔSCF (eV) | MP corr. BE (eV) | MP (fit ε) corr. BE (eV) |
|---|---|---|---|---|---|---|
| 2×2×1 | 16 | 15×15×12 | 3.50 | 187.81 | 188.56 | 188.44 |
| 4×4×2 | 128 | 8×8×6 | 1.83 | 188.10 | 188.49 | 188.43 |
| 6×6×3 | 432 | 5×5×4 | 1.23 | 188.22 | 188.49 | 188.45 |
| Extrapolated values: | | | | 188.42 | 188.44 | 188.44 |
| Experimental dielectric constant = 4.67, fitted dielectric constant = 5.49 | | | | | | |

**N 1s in hex-BN**

| Supercell | Atoms | k-grid | $q^2\alpha/2L$ (eV) | ΔSCF (eV) | MP corr. BE (eV) | MP (fit ε) corr. BE (eV) |
|---|---|---|---|---|---|---|
| 2×2×1 | 16 | 15×15×12 | 3.50 | 395.54 | 396.28 | 396.42 |
| 4×4×2 | 128 | 8×8×6 | 1.83 | 395.96 | 396.35 | 396.42 |
| 6×6×3 | 432 | 5×5×4 | 1.23 | 396.11 | 396.37 | 396.42 |
| Extrapolated values: | | | | 396.39 | 396.42 | 396.42 |
| Experimental dielectric constant = 4.67, fitted dielectric constant = 3.95 | | | | | | |

**C 1s in diamond**

| Supercell | Atoms | k-grid | $q^2\alpha/2L$ (eV) | ΔSCF (eV) | MP corr. BE (eV) | MP (fit ε) corr. BE (eV) |
|---|---|---|---|---|---|---|
| 1×1×1 | 2 | 12×12×12 | 6.44 | 280.93 | 282.06 | 282.66 |
| 2×2×2 | 16 | 6×6×6 | 4.29 | 283.11 | 283.86 | 284.27 |
| 3×3×3 | 54 | 4×4×4 | 3.00 | 283.66 | 284.19 | 284.47 |
| 4×4×4 | 128 | 3×3×3 | 2.29 | 283.81 | 284.21 | 284.43 |
| 5×5×5 | 250 | 6×6×6 | 1.86 | 283.97 | 284.30 | 284.47 |
| 6×6×6 | 432 | 6×6×6 | 1.54 | 284.05 | 284.32 | 284.46 |
| Extrapolated values: | | | | 284.43 | 284.45 | 284.46 |
| Experimental dielectric constant = 5.7, fitted dielectric constant = 3.7 | | | | | | |

**Si 2p in β-SiC**

| Supercell | Atoms | k-grid | $q^2\alpha/2L$ (eV) | ΔSCF (eV) | MP corr. BE (eV) | MP (fit ε) corr. BE (eV) |
|---|---|---|---|---|---|---|
| 1×1×1 | 2 | 48×48×48 | 6.03 | 98.42 | 99.35 | 99.71 |
| 2×2×2 | 16 | 24×24×24 | 3.60 | 98.50 | 99.06 | 99.27 |
| 3×3×3 | 54 | 16×16×16 | 2.49 | 98.76 | 99.14 | 99.29 |
| 4×4×4 | 128 | 12×12×12 | 1.91 | 98.88 | 99.17 | 99.28 |
| 5×5×5 | 250 | 10×10×10 | 1.51 | 98.95 | 99.18 | 99.27 |
| Extrapolated values: | | | | 99.24 | 99.27 | 99.28 |
| Experimental dielectric constant = 6.52, fitted dielectric constant = 4.7 | | | | | | |

**C 1s in β-SiC**

| Supercell | Atoms | k-grid | $q^2\alpha/2L$ (eV) | ΔSCF (eV) | MP corr. BE (eV) | MP (fit ε) corr. BE (eV) |
|---|---|---|---|---|---|---|
| 1×1×1 | 2 | 48×48×48 | 6.03 | 279.68 | 280.61 | 280.81 |
| 2×2×2 | 16 | 24×24×24 | 3.60 | 280.82 | 281.38 | 281.50 |
| 3×3×3 | 54 | 16×16×16 | 2.49 | 281.04 | 281.42 | 281.51 |
| 4×4×4 | 128 | 12×12×12 | 1.91 | 281.15 | 281.44 | 281.51 |
| 5×5×5 | 250 | 10×10×10 | 1.51 | 281.22 | 281.45 | 281.50 |
| Extrapolated values: | | | | 281.48 | 281.50 | 281.51 |
| Experimental dielectric constant = 6.52, fitted dielectric constant = 5.33 | | | | | | |

**Si 2p in silicon**

| Supercell | Atoms | k-grid | $q^2\alpha/2L$ (eV) | ΔSCF (eV) | MP corr. BE (eV) | MP (fit ε) corr. BE (eV) |
|---|---|---|---|---|---|---|
| 1×1×1 | 2 | 36×36×36 | 5.28 | 97.45 | 97.90 | 98.46 |
| 2×2×2 | 16 | 18×18×18 | 2.94 | 98.63 | 98.88 | 99.19 |
| 3×3×3 | 54 | 12×12×12 | 2.00 | 98.80 | 98.97 | 99.19 |
| 4×4×4 | 128 | 9×9×9 | 1.51 | 98.89 | 99.02 | 99.18 |
| 5×5×5 | 250 | 7×7×7 | 1.21 | 98.96 | 99.07 | 99.20 |
| Extrapolated values: | | | | 99.17 | 99.18 | 99.19 |
| Experimental dielectric constant = 11.7, fitted dielectric constant = 5.22 | | | | | | |

# Relaxed structures

All structures were relaxed in FHI-aims using the DFT with the exchange-correlation functional SCAN and the default "tight" basis sets and integration grids. Variable-cell relaxation with fixed angles between the unit cell vectors were performed, until all forces were below 0.005 eV/Å. In some cases, numerical stability issues were observed during structural relaxation (mismatch of real and predicted energy gain between successive relaxation steps). Numerical stability issues with the SCAN functional have been previously noted, e.g. Bartok *et al.*, *J. Chem. Phys.* **150**, 161101 (2019). To overcome this issue, the numerical grids were tightened as follows: the "radial multiplier" was increased by a factor of two, one additional localized angular grid division was uncommented, and the outermost angular grid was increased to match the uncommented value. The relaxed structures are given below, in the FHI-aims geometry.in format. All quantities are given in units of Ångström.

### k-point grids used in geometry relaxation

Lithium metal: 12×12×12

Beryllium metal: 18×18×12

Sodium metal: 12×12×12

Magnesium metal: 18×18×12

Graphite: 18×18×9

BeO: 18×18×12

hex-BN: 18×18×8

Diamond: 18×18×18

β-SiC: 18×18×18

Silicon: 18×18×18

### Lithium metal

```
lattice_vector    3.48166314   -0.00000000    0.00000000
lattice_vector    0.00000000    3.48166513    0.00000000
lattice_vector   -0.00000000    0.00000000    3.48166512
atom   -0.00000000    0.00000000    0.00000000 Li
atom    1.74083158    1.74083256    1.74083256 Li
```

**Beryllium metal**

```
lattice_vector 2.26150031 0.00827131 0.00000000
lattice_vector -1.12335037 1.96244733 0.00000000
lattice_vector 0.00000000 0.00000000 3.57104216
atom 0.00188679 1.31275315 2.67828164 Be
atom 1.13626315 0.65796560 0.89276052 Be
```

**Sodium metal**

```
lattice_vector 4.19260705 -0.00000000 0.00000000
lattice_vector -0.00000000 4.19260951 0.00000000
lattice_vector 0.00000000 0.00000000 4.19260949
atom 0.00000002 0.00000002 0.00000002 Na
atom 2.09630350 2.09630473 2.09630472 Na
```

**Magnesium metal**

```
lattice_vector 3.16084026 0.01677186 0.00000000
lattice_vector -1.56577757 2.74565180 0.00000000
lattice_vector 0.00000000 0.00000000 5.16338856
atom 0.00607990 1.83830438 1.29063688 Mg
atom 1.58898278 0.92411917 3.87275156 Mg
```

**Graphite**

```
lattice_vector 1.22503480 2.12182291 0.00000000
lattice_vector 1.22503516 -2.12182275 0.00000000
lattice_vector -0.00000000 -0.00000000 -6.90943766
atom 0.00000051 0.00228806 -5.18207532 C
atom -0.00000058 -0.00228823 -1.72736234 C
atom 1.22503564 -0.70503486 -5.18207532 C
atom 1.22503436 0.70503513 -1.72736233 C
```

**BeO**

| | | | | |
|---|---|---|---|---|
| lattice_vector | 1.34620893 | 2.32221793 | -0.00000000 | |
| lattice_vector | 1.34620938 | -2.32221782 | 0.00000000 | |
| lattice_vector | -0.00000000 | -0.00000000 | -4.36284836 | |
| atom | 1.34620922 | -0.77673125 | 0.00114554 | Be |
| atom | 1.34620905 | 0.77673129 | -2.18027864 | Be |
| atom | 1.34620923 | -0.77302324 | -2.71221950 | O |
| atom | 1.34620904 | 0.77302328 | -0.53079533 | O |

**hex-BN**

| | | | | |
|---|---|---|---|---|
| lattice_vector | 2.49434294 | 0.00322099 | 0.00000000 | |
| lattice_vector | -1.24441379 | 2.16179992 | -0.00000000 | |
| lattice_vector | -0.00000000 | 0.00000000 | 6.75674636 | |
| atom | 0.03056985 | -0.01400160 | 3.37837068 | B |
| atom | -0.02873139 | 1.45627531 | 0.00000250 | B |
| atom | -0.03128564 | 0.01468785 | 0.00000250 | N |
| atom | 0.03312410 | 1.42758586 | 3.37837068 | N |

**Diamond**

| | | | | |
|---|---|---|---|---|
| lattice_vector | 2.50282191 | -0.00738214 | -0.00521996 | |
| lattice_vector | 1.24494967 | 2.17114328 | -0.00524220 | |
| lattice_vector | 1.24565517 | 0.71917935 | 2.04918084 | |
| atom | 0.62435420 | 0.36039068 | 0.25500547 | C |
| atom | 4.36907272 | 2.52254984 | 1.78371314 | C |

**β-SiC**

| | | | | |
|---|---|---|---|---|
| lattice_vector | 2.17088417 | 2.17088417 | -0.00607491 | |
| lattice_vector | -0.00607102 | 2.17089000 | 2.17089000 | |
| lattice_vector | 2.17088420 | -0.00607489 | 2.17088420 | |
| atom | -0.00056996 | -0.00057059 | -0.00057060 | Si |
| atom | 1.08449429 | 1.08449541 | 1.08449543 | C |

**Silicon**

```
lattice_vector    -0.00000000    2.71693088    2.71693088
lattice_vector     2.71693342   -0.00000000    2.71693342
lattice_vector     2.71693596    2.71693596    0.00000000
atom    -0.00000007    -0.00000012    0.00000019 Si
atom     1.35846741     1.35846684    1.35846588 Si
```

# Basis sets

In FHI-aims, both the integration grid and the basis functions need to be defined for each type of atom in each calculation. In this work, four types of settings were used for different atoms, as described below.

- For the atom with a core hole, the “special” basis sets given below were used. This are based on the “tight” default settings, with additional core basis functions to allow the remaining core electrons to relax in the presence of the core hole.

- For the nearest neighbours of the atom with a core hole, the “tight” default settings were used.

- For the second nearest neighbours of the atom with a core hole, the “intermediate” default settings were used.

- For all other atoms, the “light” default settings were used.

- The species defaults mentioned above (default integration grids and basis sets) refer to the ones provided with FHI-aims version 201231, originally published in Blum *et al.*, *Comput. Phys. Commun.* **180**, 2175 (2009)

- The same basis sets were always used for evaluating $E_{N\text{-}1,\mathrm{ch}}$ and $E_{N\text{-}1,\mathrm{ground}}$

## Lithium

```
################################################################################
#
#  "Core" basis functions and numerical settings for Li atom.
#  Based on "tight" defaults (V. Blum, 2009).
#
################################################################################
  species        Li_core
#     global species definitions
    nucleus             3
    mass                6.941
#
    l_hartree           6
#
    cut_pot             4.5  1.8  1.0
    basis_dep_cutoff    1e-4
#
    radial_base         29 7.0
    radial_multiplier   2
    angular_grids       specified
      division   0.4484  110
      division   0.5659  194
      division   0.6315  302
      division   0.6662  434
#      division   0.8186  590
#      division   0.9037  770
#      division   6.2760  974
#      outer_grid   974
      outer_grid  434
################################################################################
#
#  Definition of "minimal" basis
#
################################################################################
#     valence basis states
    valence      2  s   1.
#     ion occupancy
    ion_occ      1  s   2.
################################################################################
#
#  Suggested additional basis functions. For production calculations,
#  uncomment them one after another (the most important basis functions are
#  listed first).
#
#  Constructed for dimers: 1.80 A, 2.25 A, 2.75 A, 3.50 A, 4.50 A
#
################################################################################
```

```
#  "First tier" - improvements: -189.23 meV to -6.35 meV
     hydro 2 p 1.6
     hydro 2 s 2
     hydro 3 d 2.6
#  "Second tier" - improvements: -4.69 meV to -0.41 meV
     hydro 3 p 4.6
     hydro 2 p 1.8
     hydro 3 s 6.2
     hydro 4 d 4.7
     hydro 4 f 4.1
#  "Third tier" - improvements: -0.20 meV to -0.15 meV
#     hydro 4 d 0.95
#     hydro 3 p 6.2
#     hydro 3 s 1.7

#  Additional basis functions for atom with a core hole
    hydro 1 s 4.0
    hydro 1 s 6.0
    hydro 2 s 5.0
```

## Beryllium

```
################################################################################
#
#  "Core" basis functions and numerical settings for Be atom.
#  Based on "tight" defaults (V. Blum, 2009).
#
################################################################################
  species        Be_core
#     global species definitions
    nucleus             4.0
    mass                9.012182
#
    l_hartree           6
#
    cut_pot             4.0  2.0  1.0
    basis_dep_cutoff    1e-4
#
    radial_base         31 7.0
    radial_multiplier   2
    angular_grids       specified
      division   0.4283  110
      division   0.4792  194
      division   0.5061  302
      division   0.7227  434
#      division   0.8724  590
#      division   0.9555  770
#      division   2.9770  974
#      outer_grid   974
      outer_grid  434
################################################################################
#
#  Definition of "minimal" basis
#
################################################################################
#     valence basis states
    valence      2  s   1.999
    valence      2  p   0.001
#     ion occupancy
    ion_occ      2  s   1.
################################################################################
#
#  Suggested additional basis functions. For production calculations,
#  uncomment them one after another (the most important basis functions are
#  listed first).
#
#  Constructed for dimers: 1.75 A, 2.0 A, 2.375 A, 3.00 A, 4.00 A
#
```

```
################################################################################
#  "First tier" - improvements: -677.26 meV to -34.75 meV
     ionic 2 p auto
     hydro 3 s 2.9
     hydro 3 d 3.5
#  "Second tier" - improvements: -16.34 meV to -1.26 meV
     hydro 3 p 3.1
     hydro 4 d 4.7
     hydro 3 p 2.4
     hydro 4 f 7.6
     hydro 2 s 2.9
#  "Third tier" - improvements: -0.27 meV to -0.05 meV
#     hydro 2 p 8.2
#     hydro 5 g 10.8
#     hydro 4 f 7
#     hydro 3 s 2.3
#     hydro 4 d 3.8

# Additional basis functions for atom with a core hole
    hydro 1 s 5.0
    hydro 1 s 7.0
    hydro 2 s 6.0
```

## Boron

```
################################################################################
#
#  "Core" basis functions and numerical settings for B atom.
#  Based on "tight" defaults (V. Blum, 2009).
#
################################################################################
  species        B_core
#     global species definitions
    nucleus             5.0
    mass                10.811
#
    l_hartree           6
#
    cut_pot             4.0  2.0  1.0
    basis_dep_cutoff    1e-4
#
    radial_base         32 7.0
    radial_multiplier   2
    angular_grids       specified
      division   0.3742  110
      division   0.5197  194
      division   0.5753  302
      division   0.7664  434
#      division   0.8392  770
#      division   1.6522  974
#      outer_grid   974
      outer_grid  434
################################################################################
#
#  Definition of "minimal" basis
#
################################################################################
#     valence basis states
    valence      2  s   2.
    valence      2  p   1.0
#     ion occupancy
    ion_occ      2  s   1.
################################################################################
#
#  Suggested additional basis functions. For production calculations,
#  uncomment them one after another (the most important basis functions are
#  listed first).
#
#  Constructed for dimers: 1.25 A, 1.625 A, 2.5 A, 3.5 A
#
################################################################################
```

```
#  "First tier" - improvements: -710.52 meV to -92.39 meV
     hydro 2 p 1.4
     hydro 3 d 4.8
     hydro 2 s 4
#  "Second tier" - improvements: -33.88 meV to -2.20 meV
     hydro 4 f 7.8
     hydro 3 p 4.2
     hydro 3 s 3.3
     hydro 5 g 11.2
     hydro 3 d 5.4
#  "Third tier" - improvements: -1.28 meV to -0.36 meV
     hydro 2 p 4.7
     hydro 2 s 8.4
     hydro 4 d 5.8
#  "Fourth tier" - improvements: -0.25 meV to -0.12 meV
#     hydro 3 p 2.2
#     hydro 3 s 3
#     hydro 4 f 9.8
#     hydro 5 g 12.8
#     hydro 4 d 10
#  Further functions
#     hydro 4 f 14
#     hydro 3 p 12.4

# Additional basis functions for atom with a core hole
hydro 1 s 9.0
hydro 1 s 7.0
hydro 1 s 3.0
hydro 2 s 5.0
hydro 2 p 6.0
```

## Carbon

```
################################################################################
#
#  "Core" basis functions and numerical settings for C atom.
#  Based on "tight" defaults (V. Blum, 2009).
#
################################################################################
  species        C_core
#     global species definitions
    nucleus             6.0
    mass                12.0107
#
    l_hartree           6
#
    cut_pot             4.0  2.0  1.0
    basis_dep_cutoff    1e-4
#
    radial_base         34 7.0
    radial_multiplier   2
    angular_grids specified
      division   0.2187   50
      division   0.4416  110
      division   0.6335  194
      division   0.7727  302
      division   0.8772  434
#      division   0.9334  590
#      division   0.9924  770
#      division   1.0230  974
#      division   1.5020 1202
#     outer_grid  974
      outer_grid  434
################################################################################
#
#  Definition of "minimal" basis
#
################################################################################
#     valence basis states
    valence      2  s   2.
    valence      2  p   2.0
#     ion occupancy
    ion_occ      2  s   1.
    ion_occ      2  p   1.
################################################################################
#
#  Suggested additional basis functions. For production calculations,
#  uncomment them one after another (the most important basis functions are
#  listed first).
```

```
#
#  Constructed for dimers: 1.0 A, 1.25 A, 1.5 A, 2.0 A, 3.0 A
#
################################################################################
#  "First tier" - improvements: -1214.57 meV to -155.61 meV
     hydro 2 p 1.7
     hydro 3 d 6
     hydro 2 s 4.9
#  "Second tier" - improvements: -67.75 meV to -5.23 meV
     hydro 4 f 9.8
     hydro 3 p 5.2
     hydro 3 s 4.3
     hydro 5 g 14.4
     hydro 3 d 6.2
#  "Third tier" - improvements: -2.43 meV to -0.60 meV
     hydro 2 p 5.6
     hydro 2 s 1.4
     hydro 3 d 4.9
     hydro 4 f 11.2
#  "Fourth tier" - improvements: -0.39 meV to -0.18 meV
#     hydro 2 p 2.1
#     hydro 5 g 16.4
#     hydro 4 d 13.2
#     hydro 3 s 13.6
#     hydro 4 f 17.6
#  Further basis functions - improvements: -0.08 meV and below
#     hydro 3 s 2
#     hydro 3 p 6
#     hydro 4 d 20

# Additional basis functions for atom with a core hole
     hydro 1 s 10.0
     hydro 1 s 8.0
     hydro 1 s 4.0
     hydro 2 s 6.0
```

## Nitrogen

```
################################################################################
#
#  "Core" basis functions and numerical settings for N atom.
#  Based on "tight" defaults (V. Blum, 2009).
#
################################################################################
  species        N_core
#     global species definitions
    nucleus             7
    mass                14.0067
#
    l_hartree           6
#
    cut_pot             4.0  2.0  1.0
    basis_dep_cutoff    1e-4
#
    radial_base         35 7.0
    radial_multiplier   2
    angular_grids       specified
      division   0.1841   50
      division   0.3514  110
      division   0.5126  194
      division   0.6292  302
      division   0.6939  434
#      division   0.7396  590
#      division   0.7632  770
#      division   0.8122  974
#      division   1.1604 1202
#      outer_grid  974
      outer_grid  434
################################################################################
#
#  Definition of "minimal" basis
#
################################################################################
#     valence basis states
    valence      2  s   2.
    valence      2  p   3.
#     ion occupancy
    ion_occ      2  s   1.
    ion_occ      2  p   2.
################################################################################
#
#  Suggested additional basis functions. For production calculations,
#  uncomment them one after another (the most important basis functions are
#  listed first).
```

```
#
#  Constructed for dimers: 1.0 A, 1.1 A, 1.5 A, 2.0 A, 3.0 A
#
################################################################################
#  "First tier" - improvements: -1193.42 meV to -220.60 meV
     hydro 2 p 1.8
     hydro 3 d 6.8
#     hydro 3 s 5.8
#  "Second tier" - improvements: -80.21 meV to -6.86 meV
     hydro 4 f 10.8
#     hydro 3 p 5.8
     hydro 1 s 0.8
     hydro 5 g 16
     hydro 3 d 4.9
#  "Third tier" - improvements: -4.29 meV to -0.53 meV
     hydro 3 s 16
     ionic 2 p auto
     hydro 3 d 6.6
     hydro 4 f 11.6
#  "Fourth tier" - improvements: -0.75 meV to -0.25 meV
#     hydro 2 p 4.5
#     hydro 2 s 2.4
#     hydro 5 g 14.4
#     hydro 4 d 14.4
#     hydro 4 f 16.8
# Further basis functions - -0.21 meV and below
#     hydro 3 p 14.8
#     hydro 3 s 4.4
#     hydro 3 d 19.6
#     hydro 5 g 12.8

# Additional basis functions for atom with a core hole
     hydro 1 s 11.0
     hydro 1 s 9.0
     hydro 1 s 5.0
     hydro 2 s 8.0
     hydro 2 s 10.0
     hydro 2 p 6.5
     hydro 3 s 6.2
     hydro 3 p 6.2
```

## Oxygen

```
################################################################################
#
#  "Core" basis functions and numerical settings for O atom.
#  Based on "tight" defaults (V. Blum, 2009).
#
################################################################################
  species        O_core
#     global species definitions
    nucleus             8
    mass                15.9994
#
    l_hartree           6
#
    cut_pot             4.0  2.0  1.0
    basis_dep_cutoff    1e-4
#
    radial_base         36 7.0
    radial_multiplier   2
     angular_grids specified
      division   0.1817   50
      division   0.3417  110
      division   0.4949  194
      division   0.6251  302
      division   0.8014  434
#      division   0.8507  590
#      division   0.8762  770
#      division   0.9023  974
#      division   1.2339 1202
#      outer_grid 974
      outer_grid  434
################################################################################
#
#  Definition of "minimal" basis
#
################################################################################
#     valence basis states
    valence      2  s   2.
    valence      2  p   4.
#     ion occupancy
    ion_occ      2  s   1.
    ion_occ      2  p   3.
################################################################################
#
#  Suggested additional basis functions. For production calculations,
#  uncomment them one after another (the most important basis functions are
#  listed first).
```

```
#
#  Constructed for dimers: 1.0 A, 1.208 A, 1.5 A, 2.0 A, 3.0 A
#
################################################################################
#  "First tier" - improvements: -699.05 meV to -159.38 meV
     hydro 2 p 1.8
     hydro 3 d 7.6
     hydro 3 s 6.4
#  "Second tier" - improvements: -49.91 meV to -5.39 meV
     hydro 4 f 11.6
     hydro 3 p 6.2
     hydro 3 d 5.6
     hydro 5 g 17.6
     hydro 1 s 0.75
#  "Third tier" - improvements: -2.83 meV to -0.50 meV
     ionic 2 p auto
     hydro 4 f 10.8
     hydro 4 d 4.7
     hydro 2 s 6.8
#  "Fourth tier" - improvements: -0.40 meV to -0.12 meV
#     hydro 3 p 5
#     hydro 3 s 3.3
#     hydro 5 g 15.6
#     hydro 4 f 17.6
#     hydro 4 d 14
# Further basis functions - -0.08 meV and below
#     hydro 3 s 2.1
#     hydro 4 d 11.6
#     hydro 3 p 16
#     hydro 2 s 17.2

# Additional basis functions for atom with a core hole
     hydro 1 s 12.0
     hydro 1 s 10.0
     hydro 1 s 6.0
     hydro 2 s 10.0
     hydro 2 p 8.0
     hydro 2 p 6.0
     hydro 3 d 8.0
```

### Sodium

```
################################################################################
#
#  "Core" basis functions and numerical settings for Na atom.
#  Based on "tight" defaults (V. Blum, 2009).
#
################################################################################
  species        Na_core
#     global species definitions
    nucleus             11
    mass                22.98976928
#
    l_hartree           6
#
    cut_pot             4.5          2.0  1.0
    basis_dep_cutoff    1e-4
#
    radial_base         40 7.0
    radial_multiplier   2
    angular_grids       specified
      division   0.5925  110
      division   0.7843  194
      division   1.0201  302
      division   1.1879  434
#      division   1.3799  590
#      division   1.4503  770
#      division   7.0005  974
#      outer_grid  974
      outer_grid  434
################################################################################
#
#  Definition of "minimal" basis
#
################################################################################
#     valence basis states
    valence      3  s   1.
    valence      2  p   6.
#     ion occupancy
    ion_occ      2  s   2.
    ion_occ      2  p   6.
################################################################################
#
#  Suggested additional basis functions. For production calculations,
#  uncomment them one after another (the most important basis functions are
#  listed first).
#
#  Constructed for dimers: 2.0 A, 2.5 A, 3.0 A, 3.75 A, 4.5 A
```

```
#
################################################################################
#  "First tier" - improvements: -60.09 meV to -10.02 meV
     hydro 2 p 1.2
     hydro 3 s 1.8
     hydro 3 d 3.8
#  "Second tier" - improvements: -2.94 meV to -1.27 meV
     hydro 4 p 3.1
     hydro 3 s 10
     hydro 4 f 6.2
     hydro 4 d 1.3
#  "Third tier" - improvements: -0.83 meV to -0.07 meV
#     hydro 3 d 7.8
#     hydro 3 p 2.3
#     hydro 5 g 9.6
#     hydro 4 p 0.85
#     hydro 5 f 1.8
#     hydro 2 s 0.6
#  Further basis functions that fell out of the optimization - noise level...
#     hydro 5 g 0.1
#     hydro 4 d 3.4
#     hydro 4 s 0.1

# Additional basis functions for atom with a core hole

    hydro 1 s 15.0
    hydro 1 s 13.0
    hydro 1 s  9.0
    hydro 2 s 13.5
    hydro 2 s 11.5
    hydro 2 p 10.5
    hydro 2 p  8.5
    hydro 3 d  7.0
    hydro 3 p  8.0
```

## Magnesium

```
################################################################################
#
#  "Core" basis functions and numerical settings for Mg atom.
#  Based on "tight" defaults (V. Blum, 2009).
#
################################################################################
  species        Mg_core
#     global species definitions
    nucleus             12
    mass                24.3050
#
    l_hartree           6
#
    cut_pot             5.0          2.0  1.0
    basis_dep_cutoff    1e-4
#
    radial_base         40 7.0
    radial_multiplier   2
    angular_grids       specified
      division   0.5421   50
      division   0.8500  110
      division   1.0736  194
      division   1.1879  302
      division   1.2806  434
#      division   1.4147  590
#      division   1.4867  770
#      division   1.6422  974
#      division   2.6134 1202
#      outer_grid   974
      outer_grid  434
################################################################################
#
#  Definition of "minimal" basis
#
################################################################################
#     valence basis states
    valence      3  p   0.001
    valence      3  s   1.999
#     ion occupancy
    ion_occ      2  s   2.
    ion_occ      2  p   6.
################################################################################
#
#  Suggested additional basis functions. For production calculations,
#  uncomment them one after another (the most important basis functions are
#  listed first).
```

```
#
#  Constructed for dimers: 2.125 A, 2.375 A, 2.875 A, 3.375 A, 4.5 A
#
################################################################################
#  "First tier" - improvements: -230.76 meV to -21.94 meV
     hydro 2 p 1.5
     ionic 3 d auto
     hydro 3 s 2.4
#  "Second tier" - improvements: -5.43 meV to -1.64 meV
     hydro 4 f 4.3
     hydro 2 p 3.4
     hydro 4 s 11.2
     hydro 3 d 6.2
#  "Third tier" - improvements: -0.92 meV to -0.22 meV
#     hydro 2 s 0.6
#     hydro 3 p 4.8
#     hydro 4 f 7.4
#     hydro 5 g 6.6
#     hydro 2 p 1.6
#     hydro 3 d 1.8
#  "Fourth tier" - improvements: -0.09 meV to -0.05 meV
#     hydro 4 p 0.45
#     hydro 5 g 10.4
#     hydro 2 s 12.4
#     hydro 4 d 1.7

# Additional basis functions for atom with a core hole
hydro 1 s 16.0
hydro 1 s 14.0
hydro 1 s 10.0
hydro 2 s 14.5
hydro 2 s 12.5
hydro 2 p 11.5
hydro 2 p 9.5
hydro 3 d 8.0
hydro 3 p 9.0
```

## Silicon

```
################################################################################
#
#  "Core" basis functions and numerical settings for Si atom.
#  Based on "tight" defaults (V. Blum, 2009).
#
################################################################################
  species        Si_core
#     global species definitions
    nucleus             14.
    mass                28.0855
#
    l_hartree           6
#
    cut_pot             4.0          2.0  1.0
    basis_dep_cutoff    1e-4
#
    radial_base         42 7.0
    radial_multiplier   2
    angular_grids       specified
      division   0.4121   50
      division   0.7665  110
      division   1.0603  194
      division   1.2846  302
      division   1.4125  434
#      division   1.4810  590
#      division   1.5529  770
#      division   1.6284  974
#      division   2.6016 1202
#      outer_grid   974
      outer_grid  434
################################################################################
#
#  Definition of "minimal" basis
#
################################################################################
#     valence basis states
    valence      3  s   2.
    valence      3  p   2.
#     ion occupancy
    ion_occ      3  s   1.
    ion_occ      3  p   1.
################################################################################
#
#  Suggested additional basis functions. For production calculations,
#  uncomment them one after another (the most important basis functions are
#  listed first).
```

```
#
#  Constructed for dimers: 1.75 A, 2.0 A, 2.25 A, 2.75 A, 3.75 A
#
################################################################################
#  "First tier" - improvements: -571.96 meV to -37.03 meV
     hydro 3 d 4.2
     hydro 2 p 1.4
     hydro 4 f 6.2
     ionic 3 s auto
#  "Second tier" - improvements: -16.76 meV to -3.03 meV
     hydro 3 d 9
     hydro 5 g 9.4
     hydro 4 p 4
     hydro 1 s 0.65
#  "Third tier" - improvements: -3.89 meV to -0.60 meV
     ionic 3 d auto
     hydro 3 s 2.6
     hydro 4 f 8.4
     hydro 3 d 3.4
     hydro 3 p 7.8
#  "Fourth tier" - improvements: -0.33 meV to -0.11 meV
#     hydro 2 p 1.6
#     hydro 5 g 10.8
#     hydro 5 f 11.2
#     hydro 3 d 1
#     hydro 4 s 4.5
#  Further basis functions that fell out of the optimization - noise
#  level... < -0.08 meV
#     hydro 4 d 6.6
#     hydro 5 g 16.4
#     hydro 4 d 9

# Additional basis functions for atom with a core hole

     hydro 2 p 15.0
     hydro 2 p 12.0
     hydro 2 p 5.0
     hydro 2 s 14.0
     hydro 1 s 16.0
     hydro 1 s 9.0
```

## Sample `control.in` files

Below, the contents of the `control.in` files, excluding the species definitions, for the calculation of the C 1s core electron binding energy in a 3×3×3 supercell of β-SiC are given. In particular:

- The charge_1 `control.in` file is used to calculate the total energy of the ground state of the N-1 electron system

- The init_part_1 and init_part_2 `control.in` files are used in successive runs to localize a core orbital onto a particular atom, and next, to create a localized core hole. In these runs, the nuclear charge of the "target" atom for localizing a core hole is increased by 0.1 e. In init_part_1, restart files are written. In init_part_2, restart files are read in and written out.

- The hole_run `control.in` file is used to calculate the total energy of the core hole state. In hole_run, restart files are read in.

- The point_charge_in_a_box `control.in` file is used to calculate the total energy of a system with just a point charge in a periodic box, with a uniform compensating background. This value is used for applying the Makov-Payne correction. In practice, the point charge is artificially created by inserting a hydrogen atom with the electron removed (except for a tiny fraction of an electron as the present version of FHI-aims does not permit calculations with an electron count of exactly zero.)

### charge_1 `control.in`

```
xc                     dfauto scan
spin                   collinear
default_initial_moment 0.0
relativistic           zora scalar 1e-12

k_grid                 16 16 16

preconditioner         kerker off

override_illconditioning .true.

charge                 1.0
```

### init_part_1 control.in

```
xc                      dfauto scan
spin                    collinear
default_initial_moment  0.0
relativistic            zora scalar 1e-12

k_grid                  16 16 16

restart_write_only      restart_file
restart_save_iterations 20
KS_method               serial

preconditioner          kerker off

override_illconditioning .true.

charge                  0.1
```

### init_part_2 control.in

```
xc                      dfauto scan
spin                    collinear
default_initial_moment  0.0
relativistic            zora scalar 1e-12

k_grid                  16 16 16

restart                 restart_file
KS_method               serial

preconditioner          kerker off

override_illconditioning .true.

charge                  1.1
force_occupation_projector 28 1 0.0 28 54
sc_iter_limit           1
```

**hole_run control.in**

```
xc                      dfauto scan
spin                    collinear
default_initial_moment 0.0
relativistic            zora scalar 1e-12

k_grid                  16 16 16

restart_read_only       restart_file
KS_method               serial

preconditioner          kerker off

override_illconditioning .true.

charge                  1.0
force_occupation_projector 28 1 0.0 28 54

output                  mulliken
```

**point_charge_in_a_box control.in**

```
xc                       dfauto scan
spin                     none
relativistic             none
KS_method                serial

charge                   0.99999999

k_grid                   1 1 1
```
